# Supplementary material for: From RAG to RICHES: Retrieval Interlaced with Sequence Generation
Source: arXiv:2407.00361 source file (2024-06-29)
Supplement: Supplementary file 1 [file additional_baselines.tex]

\begin{table*}[ht]
\begin{center}

\begin{tabular}{ll|cc}
\toprule
\multirow{2}{*}{Retriever} & \multirow{2}{*}{Answerer}  & \multicolumn{2}{c}{Hotpot} \\
& &  F1 & AutoAIS \\ 
\midrule
Decomp & Flan-T5-xxl  & 22.1 & - \\
\midrule
\multicolumn{4}{l}{\loci{}}
\llmm{}   & None  & 41.0 & 36.5 \\
\end{tabular}
\caption{Comparison of conventional Iterative retrieval methods \textit{Decomp} \citep{khot2022decomposed} with \loci{}}
\label{tab:additional_baseline}
\end{center}
\end{table*}
